# Supplementary material for: Learning Support and Trivial Prototypes for Interpretable Image Classification
Source: arXiv:2301.04011 source file (2023-10-22)
Supplement: Supplementary file 1 [file supplement_backup.tex]

\documentclass[10pt,twocolumn,letterpaper]{article}
\usepackage{iccv}
\usepackage{times}
\usepackage{epsfig}
\usepackage{graphicx}
\usepackage{amsmath}
\usepackage{amssymb}

\usepackage{booktabs}
\usepackage{multirow}
\usepackage{algorithm2e}

\usepackage{makecell}

% Include other packages here, before hyperref.

% If you comment hyperref and then uncomment it, you should delete
% egpaper.aux before re-running latex.  (Or just hit 'q' on the first latex
% run, let it finish, and you should be clear).
\usepackage[pagebackref=true,breaklinks=true,letterpaper=true,colorlinks,bookmarks=false]{hyperref}

\newcommand{\chong}[1]{{\color{blue}[chong]: #1}}
\newcommand{\gustavo}[1]{{\color{red}[gustavo]: #1}}

% \iccvfinalcopy % *** Uncomment this line for the final submission

\def\iccvPaperID{4144} % *** Enter the ICCV Paper ID here
\def\httilde{\mbox{\tt\raisebox{-.5ex}{\symbol{126}}}}

% Pages are numbered in submission mode, and unnumbered in camera-ready
\ificcvfinal\pagestyle{empty}\fi

\begin{document}

%%%%%%%%% TITLE
\title{Learning Support and Trivial Prototypes for Interpretable Image Classification (Supplementary Material)}

\author{First Author\\
Institution1\\
Institution1 address\\
{\tt\small firstauthor@i1.org}
% For a paper whose authors are all at the same institution,
% omit the following lines up until the closing ``}''.
% Additional authors and addresses can be added with ``\and'',
% just like the second author.
% To save space, use either the email address or home page, not both
\and
Second Author\\
Institution2\\
First line of institution2 address\\
{\tt\small secondauthor@i2.org}
}

\maketitle
% Remove page # from the first page of camera-ready.
\ificcvfinal\thispagestyle{empty}\fi




%%%%%%%%% BODY TEXT
\section{Training Details}
\label{sec:traindetails}

In our experiments, the proposed ST-ProtoPNet method is trained with Adam \cite{kingma2014adam} optimiser. 
The training process starts from a warm-up stage for 5 epochs, where the pre-trained CNN backbone is frozen and we only optimise the parameters of add-on layers and prototype layers, using a learning rate of $3 \times 10^{-3}$.
Then, we jointly train the CNN backbone, add-on layers, and prototype layers, where the learning rate for the CNN backbone is chosen as $1 \times 10^{-4}$ (CUB \cite{wah2011caltech}), $1 \times 10^{-4}$ (Cars \cite{krause20133d}), $1 \times 10^{-5}$ (Dogs \cite{khosla2011novel}). 
In the third stage of fully-connected (FC) layer optimisation, we utilise a learning rate of $1 \times 10^{-4}$ for 10 iterations. 
In cropped CUB and cropped Cars datasets, we decrease the learning rate by a factor of 0.2 per 2 epochs and use a weight decay ($5 \times 10^{-4}$ for VGG and ResNet, $1 \times 10^{-3}$ for DenseNet) on the CNN backbone and add-on layers. 
In full CUB, we decrease the learning rate by a factor of 0.2 per 20 epochs, a weight decay of $1 \times 10^{-4}$ is applied on all CNN backbones and add-on layers. 
In full Dogs, we decrease the learning rate by a factor of 0.2 per 10 epochs, a weight decay of $5 \times 10^{-4}$ is applied on all CNN backbones and add-on layers. 
For cropped CUB and cropped Cars, the two $1 \times 1$ convolutional layers in the add-on layers are activated by a tanh function, as a form of normalisation.

Note that, during training we alternate the optimisation of each branch of our ST-ProtoPNet among mini-batches, where we observe that our method only introduces marginal extra computational burden and does not require much additional training time to converge since the CNN backbone is shared and optimised by both branches.  

% We performed prototype projection and last layer optimisation at epoch 40 and epoch 50.
% We trained each ST-ProtoPNet for 80 epochs.  

We implemented our ST-ProtoPNet method with Pytorch \cite{paszke2019pytorch} framework and performed experiments on a machine with 4 NVIDIA GeForce RTX 3090 GPUs.


\section{Additional Results on Cars and Dogs}
\label{sec:additionalresults}

In Tables \ref{tab:interprlevel_cars} and \ref{tab:interprlevel_dogs}, we demonstrate the classification results of deep-learning based methods that have different levels of interpretability on Stanford Cars and Stanford Dogs datasets, respectively. 

As can be observed in Table \ref{tab:interprlevel_cars}, an ensemble of three ST-ProtoPNets (based on VGG19, ResNet34, and DenseNet121) reaches a high accuracy of 93.8\% on Stanford Cars, outperforming the three ensembled TesNet method (93.1\%) that uses the same CNN backbones. 
Notice that our three ensembled ST-ProtoPNet also exceeds the three ensembled ProtoPNet, ProtoTree, and ProtoPool methods by a margin of at least 2.4\%. 
Additionally, the ensemble of five ST-ProtoPNets, based on VGG19, ResNet34, ResNet152, DenseNet121, and DenseNet161, achieves the best classification accuracy of 94.1\%. 

In Table \ref{tab:interprlevel_dogs}, we can see that a single ResNet152 based ST-ProtoPNet model has a high accuracy of 87.2\% on full Stanford Dogs. 
An ensemble of three ST-ProtoPNets, based on ResNet50, ResNet152, and DenseNet161, performs better than other three ensembled methods utilising the same CNN backbones, e.g., ProtoPNet and Deformable ProtoPNet. 
The ensemble of five ST-ProtoPNets, using VGG19, ResNet50, ResNet152, DenseNet121, and DenseNet161, obtains the state-of-the-art classification accuracy of 88.7\%, surpassing other competing methods that are also based on an ensemble of five models, e.g., ProtoPNet and Deformable ProtoPNet. 


\begin{table}[]
\setlength{\tabcolsep}{1.0 mm}
\resizebox{\linewidth}{!}{


\begin{tabular}{llc} 
\hline
Interpretability level                             & Method                & Accuracy       \\ 
\hline
None                                               & B-CNN \cite{lin2015bilinear}                 & 91.3           \\ 
\hline
Object-level attention                             & CSG \cite{liang2020training}                   & 91.6           \\ 
\hline
\multirow{3}{*}{Part-level attention}              & MA-CNN \cite{zheng2017learning}               & 92.8           \\
                                                  & RA-CNN \cite{fu2017look}               & 92.5           \\
                                                  & TASN \cite{zheng2019looking}                 & \textbf{93.8}  \\ 
\hline
\multirow{9}{*}{Part-level attention + Prototypes} & Region \cite{huang2020interpretable}               & 90.9           \\
                                                  & ProtoPNet* \cite{chen2019looks}           & 91.4           \\
                                                  & ProtoTree* \cite{nauta2021neural}           & 90.5           \\
                                                  & TesNet* \cite{wang2021interpretable}              & 93.1           \\
                                                  & ProtoPool* \cite{rymarczyk2022interpretable}           & 91.1           \\
                                                  & ST-ProtoPNet* (ours)  & 93.8           \\
                                                  & ProtoTree** \cite{nauta2021neural}          & 91.5           \\
                                                  & ProtoPool** \cite{rymarczyk2022interpretable}          & 91.6           \\
                                                  & ST-ProtoPNet** (ours) & \textbf{94.1}  \\
\hline
\end{tabular}


}
\vspace{0pt}
\caption{Classification accuracy and interpretability level of different methods on Stanford Cars. *: Ensembled of three models. **: Ensembled of five models. }
\label{tab:interprlevel_cars}
% \vspace{-5pt}
\end{table}



\begin{table}[]
\setlength{\tabcolsep}{1.0 mm}
\resizebox{\linewidth}{!}{


\begin{tabular}{llc} 
\hline
Interpretability level                                  & Method                 & Accuracy       \\ 
\hline
\multirow{2}{*}{Part-level attention}             & FCAN \cite{liu2016fully}                  & 84.2           \\
                                                  & RA-CNN \cite{fu2017look}                & 87.3           \\ 
\hline
\multirow{9}{*}{Part-level attention + Prototypes} & ProtoPNet \cite{chen2019looks}             & 79.7           \\
                                                  & Deformable ProtoPNet \cite{donnelly2022deformable}  & 86.5           \\
                                                  & ST-ProtoPNet (ours)    & 87.2           \\
                                                  & ProtoPNet* \cite{chen2019looks}            & 83.6           \\
                                                  & Deformable ProtoPNet* \cite{donnelly2022deformable} & 87.1           \\
                                                  & ST-ProtoPNet* (ours)   & 88.6           \\
                                                  & ProtoPNet** \cite{chen2019looks}           & 84.1           \\
                                                  & Deformable ProtoPNet** \cite{donnelly2022deformable} & 87.3           \\
                                                  & ST-ProtoPNet** (ours)   & \textbf{88.7}  \\
\hline
\end{tabular}


}
\vspace{0pt}
\caption{Classification accuracy and interpretability level of different methods on Stanford Dogs. *: Ensembled of three models. **: Ensembled of five models. }
\label{tab:interprlevel_dogs}
% \vspace{-10pt}
\end{table}





\section{Ablation on Coefficient $\lambda_3$}
\label{sec:lambda3}

The coefficient $\lambda_3$ in our method controls the strength of the proposed closeness loss $\ell_{cls}$ and discrimination loss $\ell_{dsc}$ for the learning of support and trivial prototypes, respectively. 
We perform an ablation experiment to study the sensitivity of our ST-ProtoPNet method to the hyperparameter $\lambda_3$.
Table \ref{tab:lambda3} shows the effect of $\lambda_3$ on the classification accuracy of our ST-ProtoPNet. 
As evident, if $\lambda_3$ is too small, other loss terms (e.g., cross-entropy, clustering, and separation) will dominate the optimisation process, which leads to performance degradation. 
However, if $\lambda_3$ is too large, other losses (particularly the cross-entropy loss) will be distracted, resulting in lower discrimination ability.
Therefore, we choose $\lambda_3$ = 1.0 in all our experiments.



\begin{table}[]
\vspace{5pt}
\setlength{\tabcolsep}{2.65 mm}
\resizebox{\linewidth}{!}{


\begin{tabular}{ccccccccc} 
\hline
$\lambda_3$        & 0 & 0.01 & 0.1 & 0.5 & 1.0 & 2.0 & 5.0 & 10.0  \\ 
\hline
Accuracy & 81.6   & 81.8     & 82.7    & 83.4    & 83.5    & 83.3    & 83.0    & 81.8      \\
\hline
\end{tabular}


}
\vspace{0pt}
\caption{Ablation to study the effect of hyperparameter $\lambda_3$ on the accuracy of our ResNet34-based ST-ProtoPNet on cropped CUB.}
\label{tab:lambda3}
% \vspace{-10pt}
\end{table}





\section{Ablation on Independent Add-on Layers}
\label{sec:addon}

In our ST-ProtoPNet method, the support and trivial ProtoPNets are branched after the CNN backbone and they have independent add-on layers. 
One may also consider using shared add-on layers, where both the support and trivial prototypes will employ the same feature maps. 
We thus design an ablation study on full CUB to compare the classification results between using independent and shared add-on layers. 
Table \ref{tab:abladdon} gives the experimental results with VGG19, ResNet50, and Dense121 as CNN backbones. 
We can observe that using independent add-on layers exhibits higher classification accuracy across different CNN backbones. 
One possible explanation is the support and trivial prototypes have distinctive characteristics that require different feature representations for classification. 


\begin{table}[]
% \vspace{5pt}
\setlength{\tabcolsep}{0.7 mm}
\resizebox{\linewidth}{!}{


\begin{tabular}{lccc} 
\hline
Method          & \multicolumn{1}{l}{VGG19} & ResNet50 & \multicolumn{1}{l}{Dense121}  \\ 
\hline
ST-ProtoPNet (shared add-on layers) & 79.2                        & 87.5     &  81.2                             \\
ST-ProtoPNet (independent add-on layers) & 80.2                      & 88.0     & 81.8                          \\
\hline
\end{tabular}


}
\vspace{0pt}
\caption{Ablation study on using independent or shared add-on layers for our ST-ProtoPNet method.}
\label{tab:abladdon}
% \vspace{-10pt}
\end{table}





\section{Effect of Prototype Pruning}
\label{sec:prune}

Prototype pruning \cite{chen2019looks} can automatically remove non-discriminative background prototypes. 
Less pruned prototypes indicate more prototypes focus on the discriminative object regions, we thus favour a smaller number of pruned prototypes. 
We conduct experiments with pruning for the support and trivial prototypes. 
Following \cite{chen2019looks}, during pruning we employ 6 nearest latent patches for each prototype and set the pruning threshold $\tau$ = 3.
In order to achieve fair comparison with the vanilla ProtoPNet \cite{chen2019looks}, we do not use the orthonormality loss $\ell_{ort}$, and add only our proposed closeness loss $\ell_{cls}$ or discrimination loss on $\ell_{dsc}$ to the vanilla ProtoPNet \cite{chen2019looks} to establish the Support ProtoPNet or Trivial ProtoPNet, respectively.
Table \ref{tab:prune} presents the experimental results on cropped CUB by using VGG19 as CNN backbone. 
As can be seen, the number of pruned support prototypes are substantially reduced, compared with that of trivial prototypes in the vanilla ProtoPNet \cite{chen2019looks} and Trivial ProtoPNet, verifying that our proposed support prototypes are less likely to be localised on background regions. 




\begin{table}[]
\vspace{5pt}
\setlength{\tabcolsep}{0.8 mm}
\resizebox{\linewidth}{!}{


\begin{tabular}{ccccc} 
\hline
Method   & \makecell[c]{Accuracy \\ before pruning}  & \makecell[c]{Accuracy \\ after pruning} & \makecell[c]{Accuracy \\ after pruning and \\ optimising last layer} & \makecell[c]{Number \\ of pruned \\ prototype}  \\ 
\hline
ProtoPNet \cite{chen2019looks}    & 78.2                    & 74.4                   & 78.0                   & 666                  \\
Trivial ProtoPNet                 & 78.6                    & 74.4                   & 78.3                   & 701                  \\
Support ProtoPNet                 & 79.7                    & 74.7                   & 79.4                   & 409                  \\
\hline
\end{tabular}


}
\vspace{0pt}
\caption{Effect of prototype pruning on different ProtoPNet methods trained on cropped CUB.}
\label{tab:prune}
% \vspace{-10pt}
\end{table}







\section{Visualisation of Object Localisation on CUB}
\label{sec:localisation}

In Fig.~\ref{fig:birdlocalisation}, we present some examples of the activation map generated by our ST-ProtoPNet and other competing methods for images from the full CUB test set. 
It can be observed that, compared with the vanilla ProtoPNet \cite{chen2019looks}, our method mainly relies on the object (i.e., bird) region instead of the background pixels. 
In addition, we also notice that our method has more activation coverage on the target object than TesNet \cite{wang2021interpretable} and Deformable ProtoPNet \cite{donnelly2022deformable}, which demonstrates that our proposed method utilises both the support and trivial prototypes to effectively capture much richer representations of the target object. 


\begin{figure}[t!]
    \centering
    \includegraphics[width=1.00\linewidth]{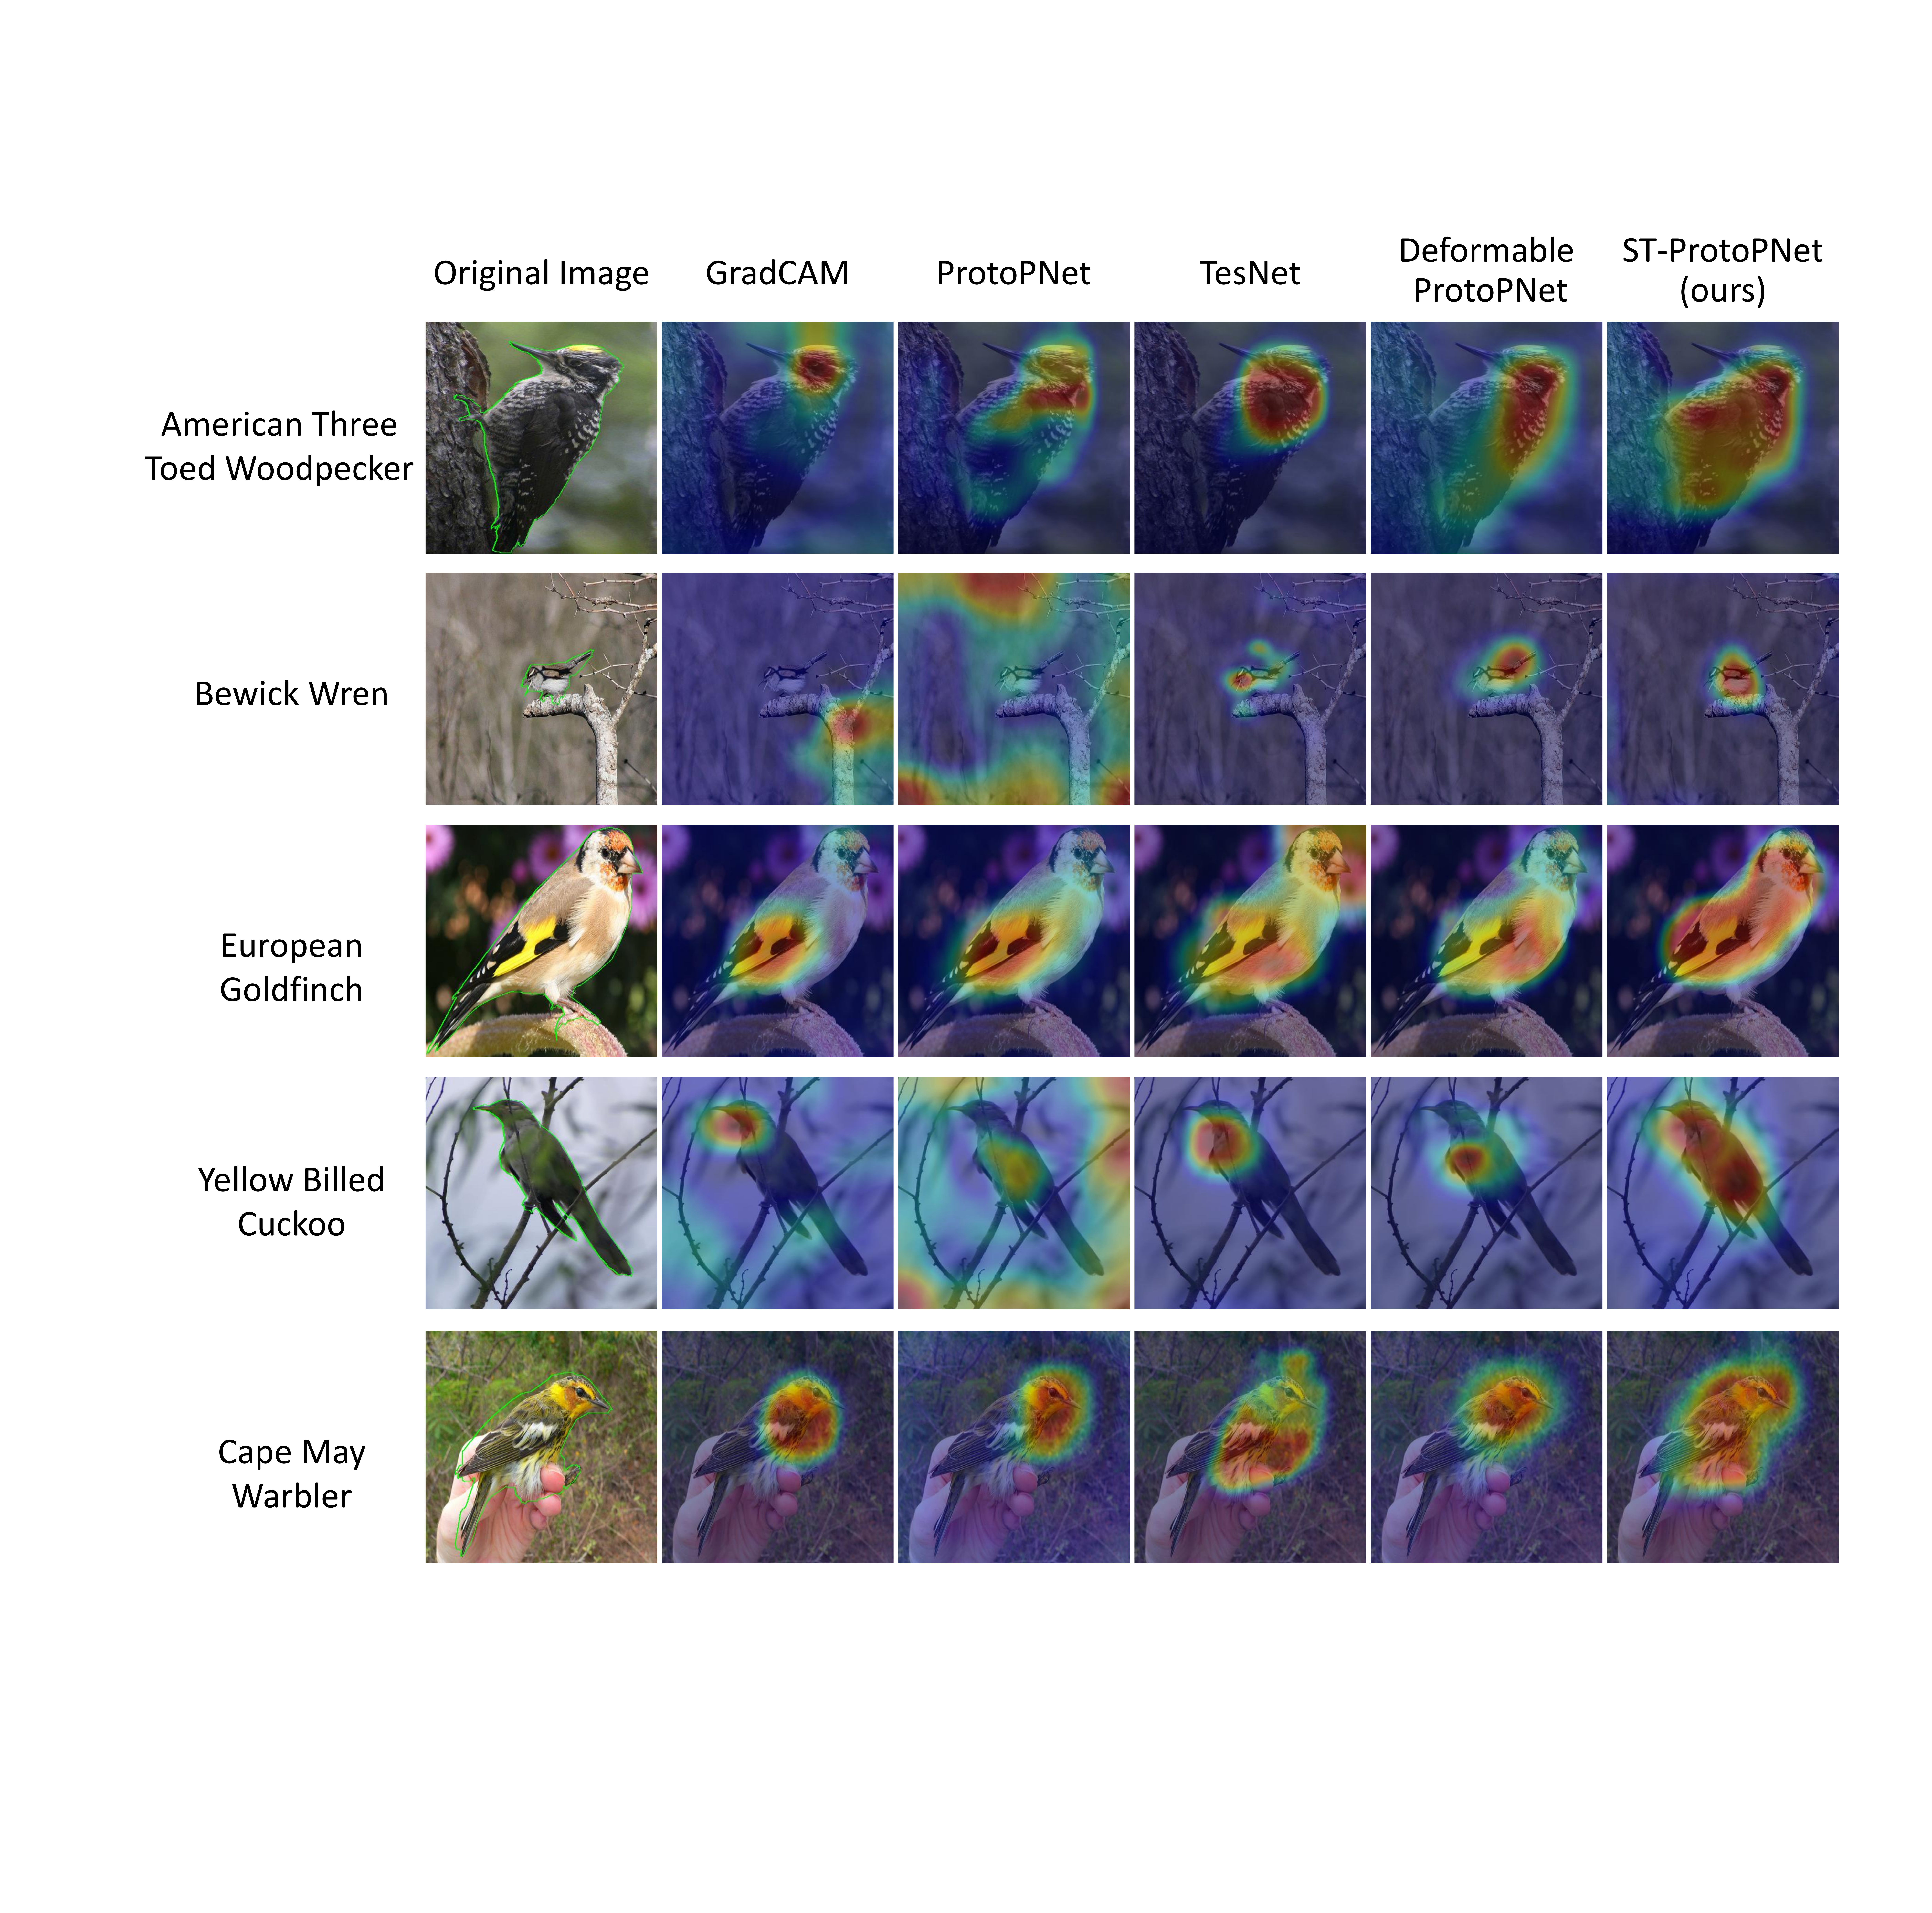}
    % \vspace{-20pt}
    \caption{Activation map for images from the full CUB test set. The bird in the original images is indicated by a green boundary outline extracted from the annotated segmentation mask. For prototype-based methods, the activation map is obtained by averaging all activation maps of the class. }
    \label{fig:birdlocalisation}
    % \vspace{10pt}
\end{figure}


\section{More Examples of Prototype Visualisation}
\label{sec:prototype}

In Fig.~\ref{fig:visualprototypescar} and \ref{fig:visualprototypesdog}, we provide more visual examples of typical prototypes learned by our top-performing models on Stanford Cars and Stanford Dogs datasets.
Specifically, we display prototypes of Dense161-based and ResNet152-based ST-ProtoPNet for Stanford Cars and Stanford Dogs, respectively.
Following previous studies \cite{chen2019looks,donnelly2022deformable}, all these prototypes are visualised by projecting onto their nearest training patch in the latent feature space. 

\subsection{Stanford Cars}

In Fig.~\ref{fig:visualprototypescar}, we demonstrate the visual prototypes of four classes (Acura RL Sedan 2012, Acura TL Sedan 2012, Acura TL Type-S 2008, and Acura TLS Sedan 2012) learn from cropped Stanford Cars dataset. 
We can note from Fig.~\ref{fig:visualprototypescar}(a) that the support prototypes mainly capture visually similar features of different classes, such as the light and front bumper. 
By contrast, the trivial prototypes in Fig.~\ref{fig:visualprototypescar}(b) are inclined to focus on not only lights but also other car parts, such as wheel, door, and window. 
For the cropped Cars dataset, the target objects of cars usually occupy a large area in the whole image, so we rarely observe background regions in trivial prototypes.


\begin{figure*}[t!]
    \centering
    \includegraphics[width=1.00\linewidth]{figures/car_prototypes.pdf}
    % \vspace{-20pt}
    \caption{Visual comparison between the support (a) and trivial (b) prototypes from cropped Stanford Cars, where each row exhibits prototypes of the same class. In each pair, the first column shows the original image with a prototype indicated in a yellow bounding box, the second column demonstrates the prototype’s corresponding activation map. }
    \label{fig:visualprototypescar}
    \vspace{10pt}
\end{figure*}



\subsection{Stanford Dogs}

In Fig.~\ref{fig:visualprototypesdog}, we demonstrate some typical prototypes of five classes (Rhodesian Ridgeback, Toy Terrier, Komondor, Rottweiter, and Dhole) from full Stanford Dogs dataset. 
It can be observed from Fig.~\ref{fig:visualprototypesdog}(a) that the support prototypes often contain similar visual patterns of different classes, e.g., dog's eye, mouth, and head. 
By contrast, trivial prototypes in Fig.~\ref{fig:visualprototypesdog}(b) are usually from dog's neck, leg, and belly (lower surface) regions. 
We also notice that two trivial prototypes capture background regions (rightmost ones of the Rottweiter and Dhole classes). 



\begin{figure*}[t!]
    \centering
    \includegraphics[width=1.00\linewidth]{figures/dog_prototypes.pdf}
    % \vspace{-20pt}
    \caption{Visual comparison between the support (a) and trivial (b) prototypes from full Stanford Dogs, where each row exhibits prototypes of the same class. In each pair, the first column shows the original image with a prototype indicated in a yellow bounding box, the second column demonstrates the prototype’s corresponding activation map. }
    \label{fig:visualprototypesdog}
    \vspace{10pt}
\end{figure*}



\section{More Examples of Interpretable Reasoning}
\label{sec:reasoning}

We provide more examples of the interpretable reasoning process of our ST-ProtoPNet method on Stanford Cars (Dense161-based) and Stanford Dogs (ResNet152-based) datasets, as illustrated in Fig.~\ref{fig:reasoningcar} and Fig.~\ref{fig:reasoningdog}. 
For each example, we display two support and trivial prototypes of the predicted class as well as the corresponding source training images where these prototypes come. 
For a testing image, the activation maps and highest similarity scores with these prototypes are also provided. 
For simplicity, we only demonstrate the prototypes, activation maps, and similarity scores contributing to the predicted class for each example. 

\subsection{Stanford Cars} 

Fig.~\ref{fig:reasoningcar} displays the interpretable reasoning of our ST-ProtoPNet method in classifying a testing car (Acura TL Type-S 2008) image. 
In each ProtoPNet branch, our method compares the testing image with training prototypes and computes the corresponding similarity scores, which is then weighted and summed to produce the classification logits.
The final classification logits is the sum of logits from both branches. 
In particular, the support prototypes are mostly active on the fog light and headlight of the car. 
Meanwhile, the trivial prototypes have high activations on the car’s window and wheel. 
In this case, the support ProtoPNet branch generates a comparably larger similarity score (17.840) in comparison with the trivial ProtoPNet branch (16.698), meaning that the testing car image is more similar to the support prototypes than the trivial ones.
We can see that the support and trivial prototypes make complementary predictions contributing to the final classification decision. 

\begin{figure}[t!]
    \centering
    \includegraphics[width=1.00\linewidth]{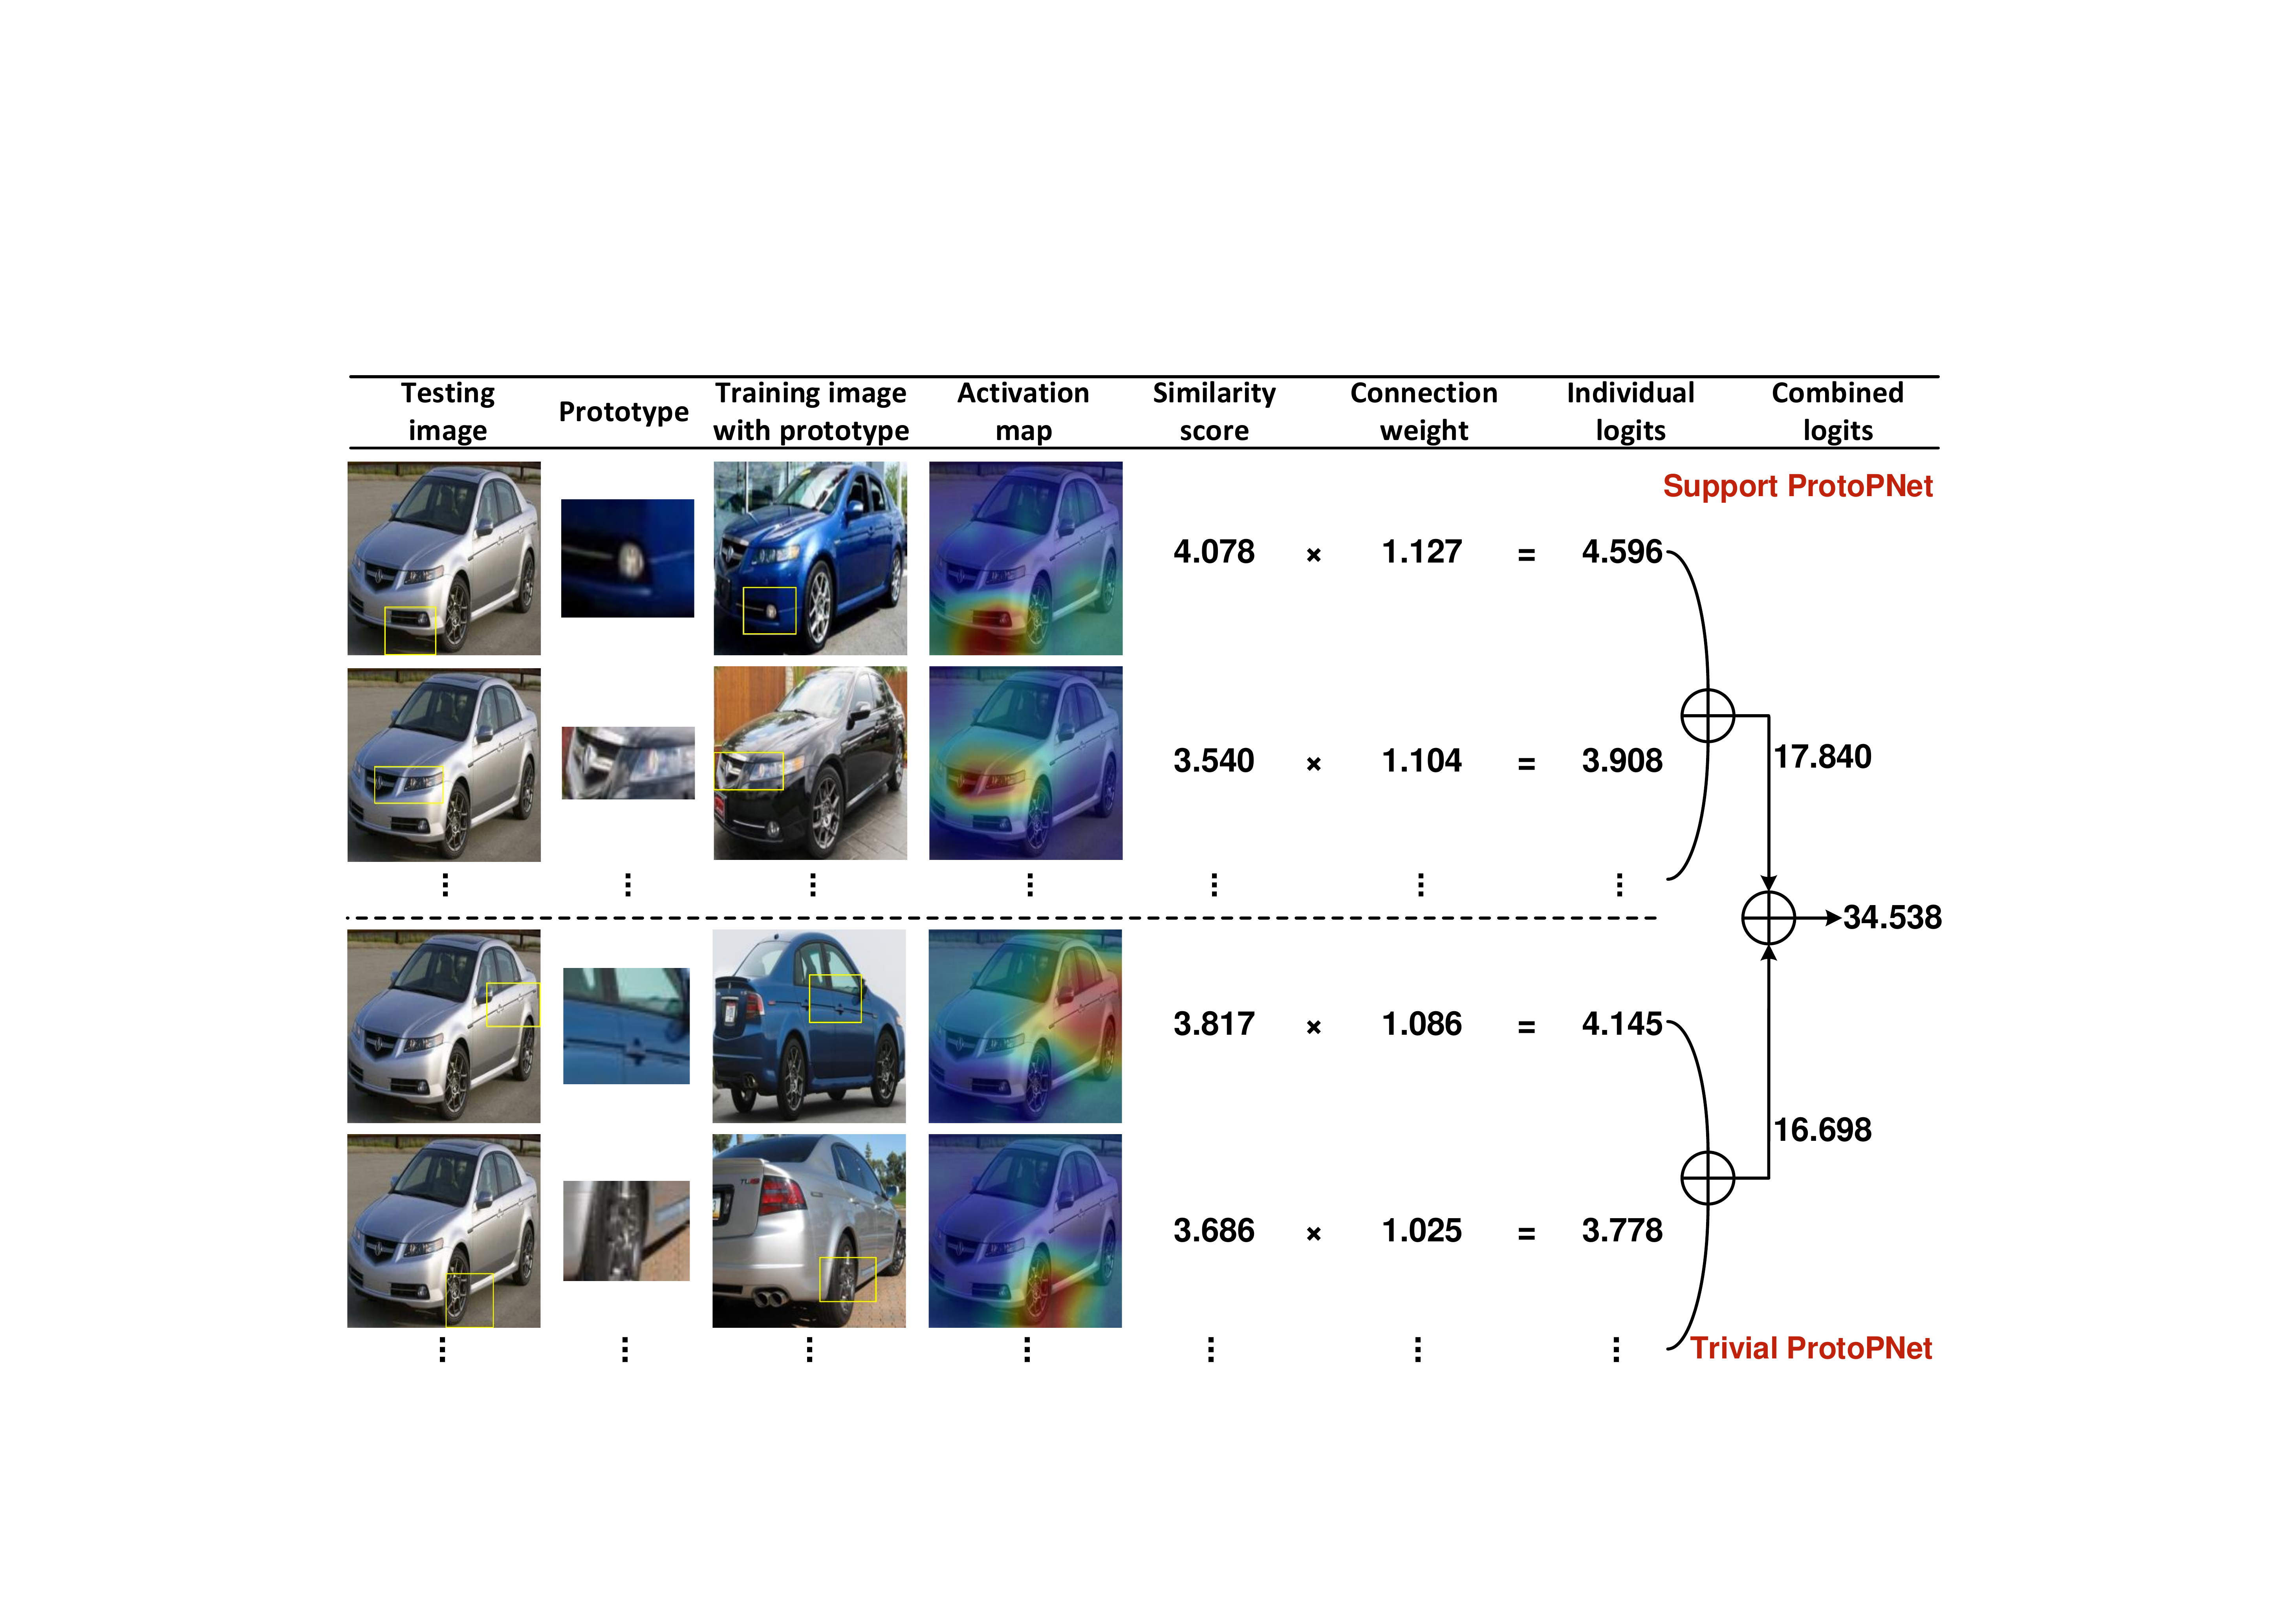}
    % \vspace{-20pt}
    \caption{An example of the interpretable reasoning of our ST-ProtoPNet for classifying a testing car (Acura TL Type-S 2008) image. }
    \label{fig:reasoningcar}
    \vspace{10pt}
\end{figure}


\subsection{Stanford Dogs}

Fig.~\ref{fig:reasoningdog} reveals the interpretable reasoning of our ST-ProtoPNet method in classifying a testing dog (Rhodesian Ridgeback) image. 
To be specific, when classifying the Rhodesian Ridgeback dog, its head is usually activated by the support prototypes while its neck and belly are often activated by the trivial prototypes. 
% In this case, the support ProtoPNet branch obtains a relatively higher similarity score (22.713) compared with the trivial branch (20.948).
We should notice that for the full Stanford Dogs dataset, we utilise cosine similarity \cite{donnelly2022deformable}, instead of projection metric \cite{wang2021interpretable} used in cropped Stanford Cars, to measure the similarity between the testing image's feature map and prototypes, so the similarity scores are within the range of [0, 1]. 
In this example, the support and trivial ProtoPNet branches obtain an accumulated similarity score of 35.902 and 35.583, respectively.
By using both support and trivial prototypes, our ST-ProtoPNet can capture richer representations of the target object (dog in this example) from different perspectives to achieve complementary interpretations.



\begin{figure}[t!]
    \centering
    \includegraphics[width=1.00\linewidth]{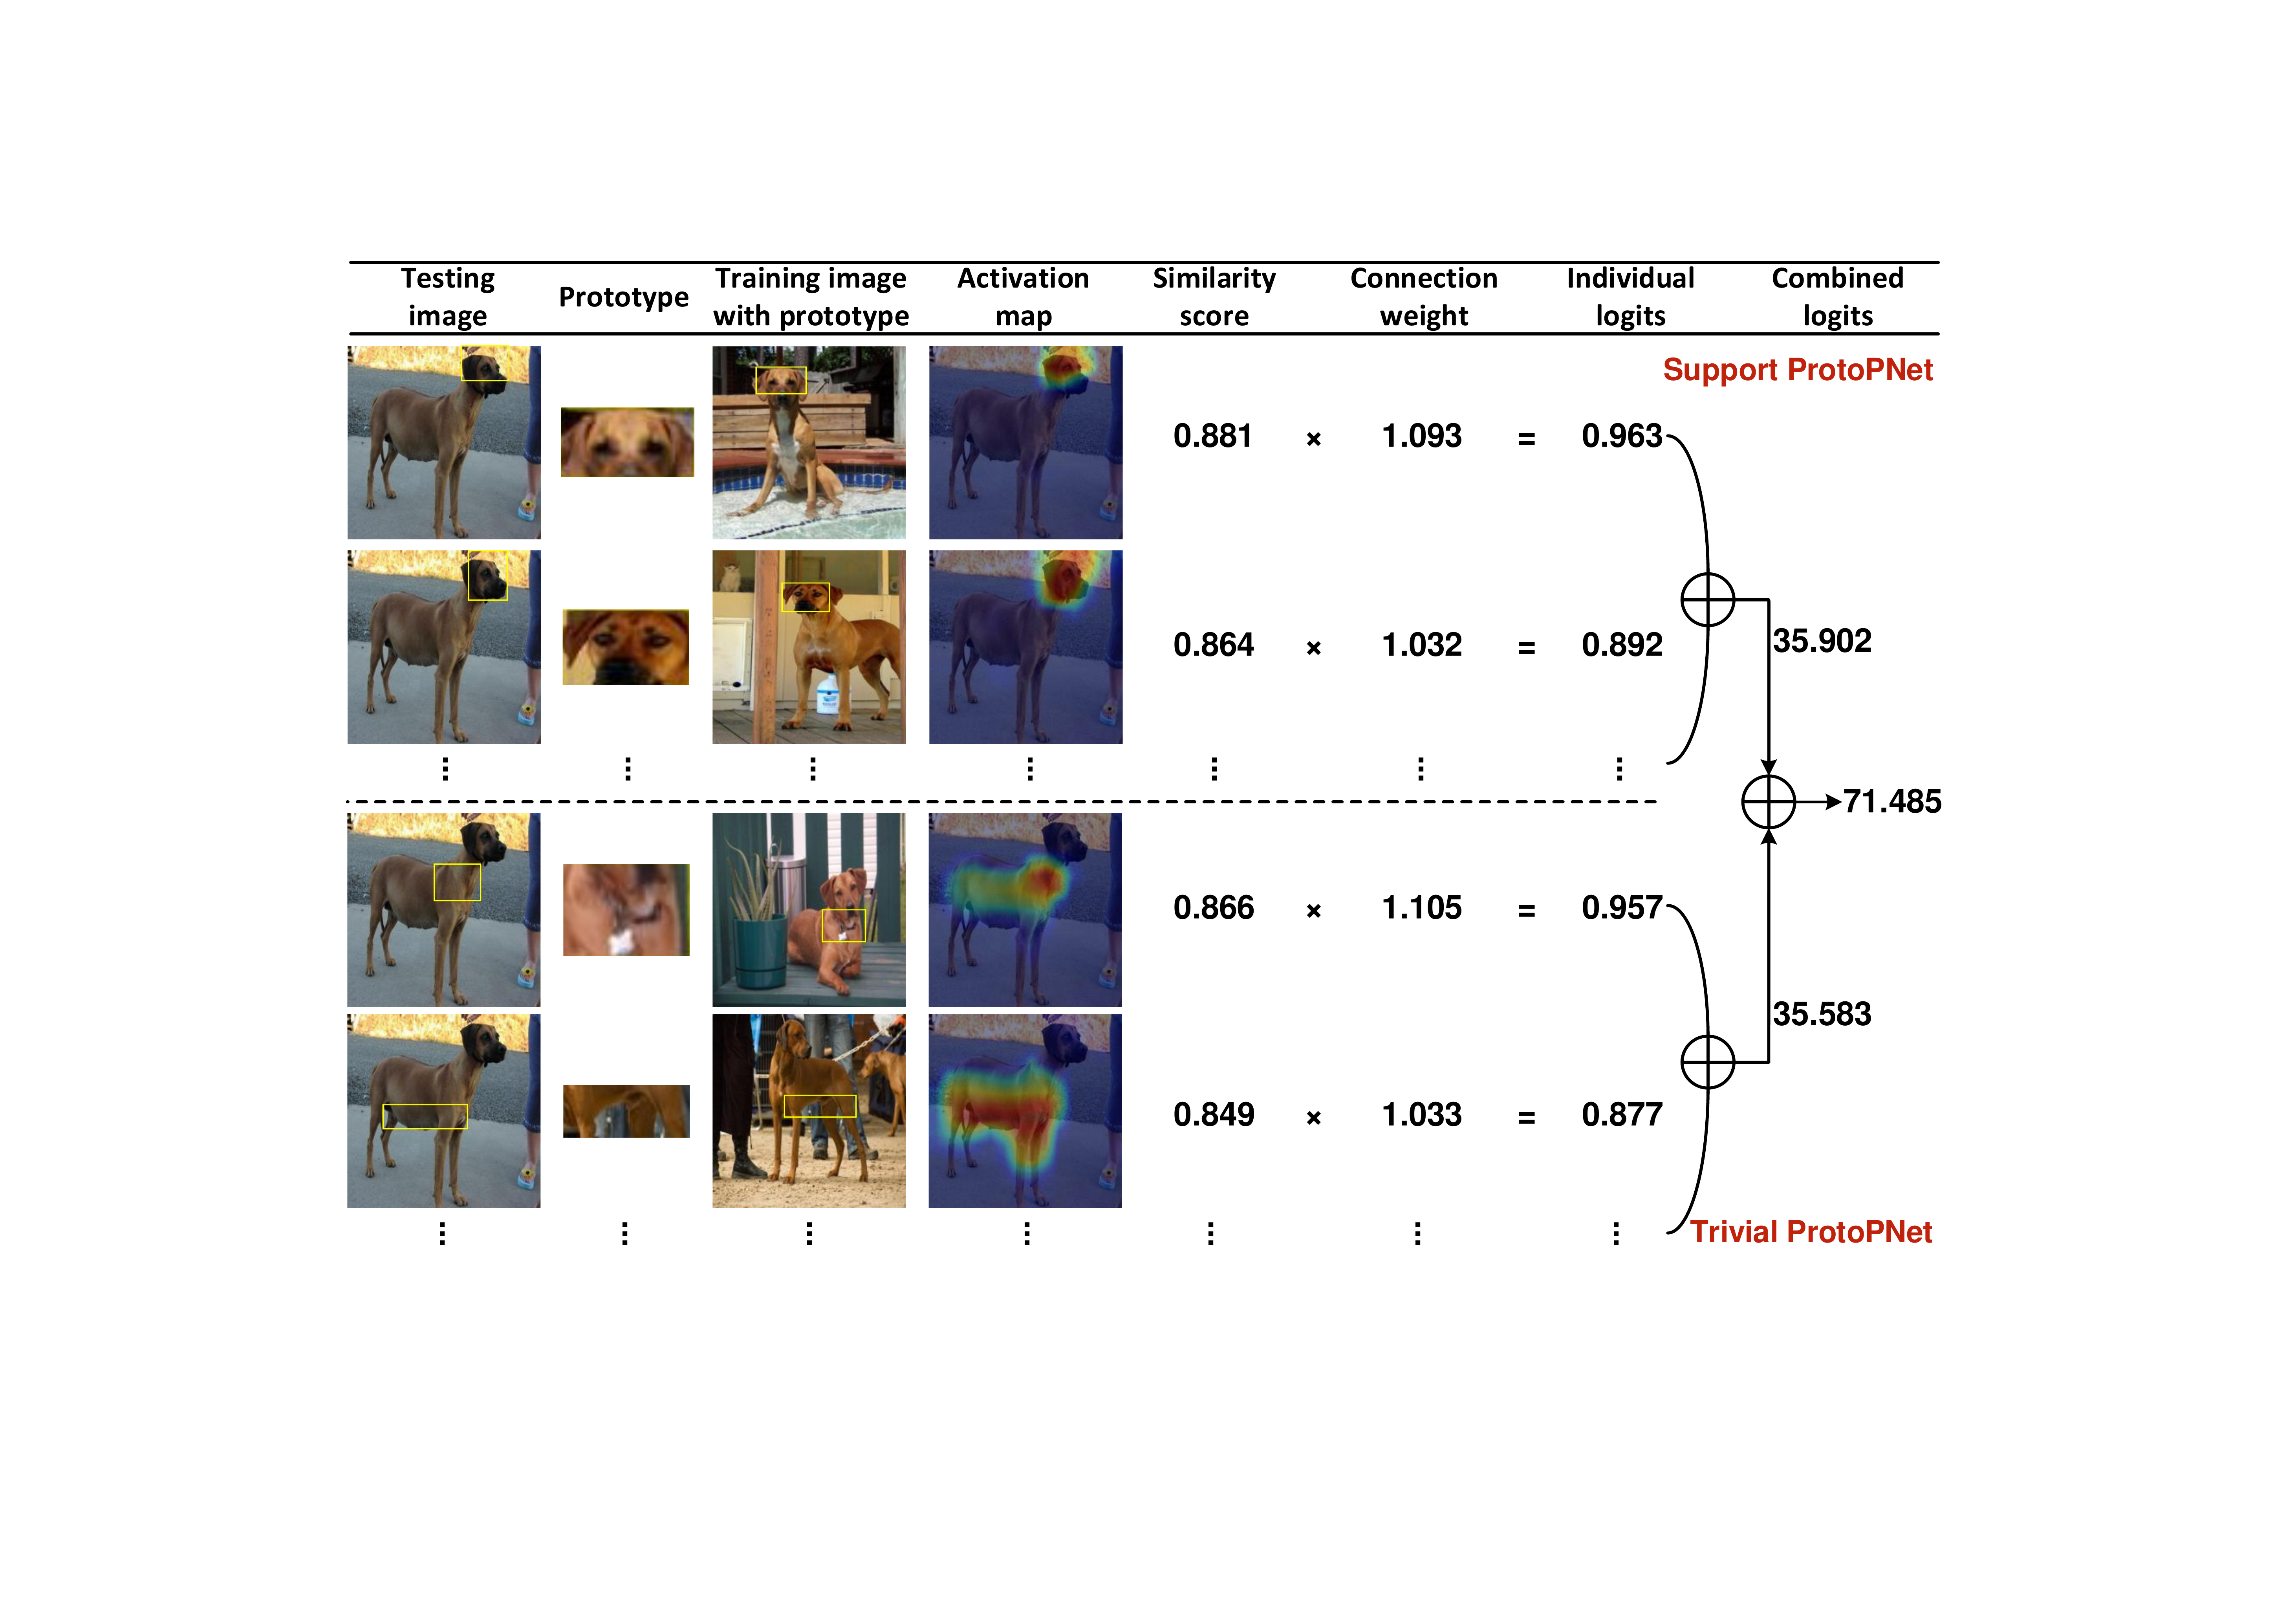}
    % \vspace{-20pt}
    \caption{An example of the interpretable reasoning of our ST-ProtoPNet for classifying a testing dog (Rhodesian Ridgeback) image. }
    \label{fig:reasoningdog}
    \vspace{10pt}
\end{figure}



% \section{Local Analysis: Finding Most Similar Prototypes to a Given Image}

% In this paper, we propose the ST-ProtoPNet method to exploit both support (i.e., hard-to-learn) and trivial (i.e., easy-to-learn) prototypes for the interpretable image classification, where the two sets of prototypes can provide complementary results. 
% In addition, our ST-ProtoPNet is a general approach that can be easily applied to existing prototype-based interpretable models. 
% One limitation for our method is that we empirically adopt the same number of support and trivial prototypes and the same total number of prototypes for each class. Given the different learning difficulties and imbalanced training samples among classes in other real-world datasets, e.g., ImageNet \cite{deng2009imagenet}, a better way to learn a flexible number of support and trivial prototypes is needed and deserves to be further investigated in our future work. 


% \section{Global Analysis: Finding Most Similar Images to a Given Prototype}

% In this paper, we mimic the behaviour of the support vectors of SVM classifier to obtain the support prototypes by forcing them to be as close as possible to the classification boundary. 
% In the future, we will formulate the learning of prototypes with gradient-based kernel computations, e.g., neural tangent kernel \cite{jacot2018neural} and path kernel \cite{domingos2020every}. 




% \clearpage

%%%%%%%%% REFERENCES
{\small
\bibliographystyle{ieee_fullname}
\bibliography{refs}
}



\end{document}
